# Supplementary material for: Construction and Elicitation of a Black Box Model in the Game of Bridge
Source: arXiv:2005.01633 source file (2022-04-04)
Supplement: Supplementary file 1 [file appendixENG.tex]

\noindent
\begin{minipage}{\linewidth}
{\footnotesize 
 \begin{lstlisting}[frame = single, caption = A complete tree learned by Tilde, label = best-tree-tilde-complete]
decision(-A,-B,-C,-D,-E)
nb(A,-F,-G),gteq(G,6)? 
+--yes: hcp(A,4)? 
|   +--yes: [pass] 2.0
|   +--no:  [bid] 57.0
+--no:  hcp(A,-H),gteq(H,16)? 
    +--yes: [bid] 6.0
    +--no:  nb(A,spade,-I),gteq(I,1)? 
        +--yes: lteq(I,1)? 
        |   +--yes: hcp(A,-J),lteq(J,5)? 
        |   |   +--yes: [pass] 11.0
        |   |   +--no:  nb(A,-K,5)? 
        |   |       +--yes: hcp(A,6)? 
        |   |       |   +--yes: [pass] 3.0
        |   |       |   +--no:  [bid] 27.0
        |   |       +--no:  [pass] 3.0
        |   +--no:  hcp(A,15)? 
        |       +--yes: [bid] 3.0
        |       +--no:  nb(A,-L,3)? 
        |           +--yes: [pass] 146.0 
        |           +--no:  hcp(A,11)? 
        |               +--yes: [bid] 3.0 
        |               +--no:  hcp(A,-M),lteq(M,6)? 
        |                   +--yes: [pass] 15.0 
        |                   +--no:  lteq(I,2)? 
        |                       +--yes: nb(A,-N,1)? 
        |                       |   +--yes: [bid] 3.0
        |                       |   +--no:  hcp(A,-O),gteq(O,11)? 
        |                       |       +--yes: [bid] 5.0
        |                       |       +--no:  [pass] 16.0
        |                       +--no:  [pass] 5.0
        +--no:  [bid] 5.0 

\end{lstlisting}
}
\end{minipage}

\noindent
\begin{minipage}{\linewidth}
{\footnotesize 
\begin{lstlisting} [frame=single,caption=All rules of an $L_2$-Aleph-induce\_max model,  label=complete-best-rules-aleph,escapechar=\%]
decision(A,4,B,C,bid) :-
   nbs(A,0).
decision(A,4,B,C,bid) :-
   hcp(A,D), gteq(D,5), nb(A,E,F), gteq(F,6), nbs(A,1).
decision(A,4,B,C,bid) :-
   hcp(A,D), gteq(D,9), nbs(A,1).
decision(A,4,B,C,bid) :-
   hcp(A,D), gteq(D,8), nb(A,E,F), gteq(F,5), nbs(A,1).
decision(A,4,B,C,bid) :-
   hcp(A,D), gteq(D,4), distribution(A,[6,4,2,1]).
decision(A,4,B,C,bid) :-
   hcp(A,D), gteq(D,8), nb(A,E,F), gteq(F,6), nbs(A,2).
decision(A,4,B,C,bid) :-
   hcp(A,D), gteq(D,13), nb(A,E,F), gteq(F,5), nbs(A,2).
decision(A,4,B,C,bid) :-
   hcp(A,D), gteq(D,10), nb(A,E,F), gteq(F,6).
decision(A,4,B,C,bid) :-
   nb(A,D,E), gteq(E,7).
decision(A,4,B,C,bid) :-
   hcp(A,D), gteq(D,14), nb(A,E,F), gteq(F,5).
decision(A,4,B,C,bid) :-
   nb(A,D,E), lteq(E,1), nbs(A,2).
decision(A,4,B,C,bid) :-
   hcp(A,D), nb(A,E,D), nb(A,F,G), gteq(G,6).
decision(A,4,B,C,bid) :-
   hcp(A,D), gteq(D,12), nb(A,E,F), lteq(F,1).
decision(A,4,B,C,bid) :-
   hcp(A,D), lteq(D,7), gteq(D,7), nb(A,E,F), gteq(F,6).
decision(A,4,B,C,bid) :-
   hcp(A,D), gteq(D,14), nbs(A,2).

\end{lstlisting}
}
\end{minipage}

\begin{table}[htb!]
  \begin{center}
    \begin{tabular}{c|c|c} % <-- Alignments: 1st column left, 2nd middle and 3rd right, with vertical lines in between
      \pmb{$L_0$} & \pmb{$L_1$} & \pmb{$L_2$}\\
      \hline
      $suit\_rep(H,Suit,Hon,Num)$ & & \\
      $distribution(H,[N,M,P,Q])$ &  & $distribution(H,[N,M,P,Q])$\\
      $nb(H,Suit,Num)$ & $nb(H,Suit,Num)$ & $nb(H,Suit,Num)$\\
      $hcp(H,Num)$ & $hcp(H,Num)$ & $hcp(H,Num)$\\
      $semibalanced(H)$ & $semibalanced(H)$ & 
      \\
      $unbalanced(H)$ & $unbalanced(H)$ & 
      \\
      $balanced(H)$ &
      $balanced(H)$ & 
      \\
      $vuln(Pos,Vul,Dlr,NS,EW)$ & $vuln(Pos,Vul,Dlr,NS,EW)$ &
      \\
      $vuln(Pos,Vul,Dlr,NS,EW)$ & $vuln(Pos,Vul,Dlr,NS,EW)$ &
      \\
      $lteq(Num,Num)$ & $lteq(Num,Num)$ &
      $lteq(Num,Num)$\\
      $gteq(Num,Num)$ & $gteq(Num,Num)$ &
      $gteq(Num,Num)$\\
      $longest\_suit(H,Suit)$ &
      $longest\_suit(H,Suit)$ &
      \\
      $shortest\_suit(H,Suit)$ &
      $shortest\_suit(H,Suit)$ &
      \\
      $major(Suit)$ &
      $major(Suit)$ &
      \\
      $minor(Suit)$ &
      $minor(Suit)$ &
      \\
      & & $nbs(H,Num)$\\
    \end{tabular}
    \caption{Predicates in the domain theories}\label{domain_theories}
  \end{center}
\end{table}

\noindent
\begin{minipage}{\linewidth}
{\footnotesize 
\begin{lstlisting} [frame=single,caption=$C_0$: Set of common rules for the 4\Ss{} bid,  label=common-4s-rules,escapechar=\%]
rule(A,1) :-
    nb_top_honor(A,B,2,[club,diamond,heart]), lteq(B,1).
rule(A,2) :-
    nb_quick_tricks_spade(A,B), lteq(B,9).
rule(A,3) :-
    hcp(A,B), gteq(B,3), lteq(B,11).
rule(A,3) :-
    hcp(A,12), nb(A,_,1), nb_top_honor(A,1,4,[spade]),
    nb_top_honor(A,0,2,[spade]).
rule(A,4) :-
    nb(A,spade,B), gteq(B,7), lteq(B,9).

\end{lstlisting}
}
\end{minipage}
